# Supplementary material for: Stream-based active learning with linear models
Source: arXiv:2207.09874 source file (2023-07-13)
Supplement: Supplementary file 1 [file 6_appendix.tex]

\section{Weighted prediction variance}\label{app:a}

In this section, we examine the impact of switching from the standard UPV to its weighted version $\text{UPV}_w$ on the learning curves of the robust bounded CDO strategies. While it may seem reasonable to use a weighted prediction variance from a theoretical standpoint, we found little compelling evidence that it improves the performance. In fact, we observed that using the $\text{UPV}_w$ actually worsens results when the initial design is free from outliers. This could be because the robust models mistakenly identify some observations as outliers, resulting in $\mathbf{W} \neq \mathbf{I}_{k}$.

\begin{figure}[h]
  \centering
  \includegraphics[width=.7\linewidth]{images/upv_w_0.00275.png}
  \caption{Comparing UPV and $\text{UPV}_w$ in the scenario with 0.275\% outliers (1000 simulations).}
  \label{fig:upv0275}
\end{figure}

\begin{figure}[h]
  \centering
  \includegraphics[width=.7\linewidth]{images/upv_w_0.01.png}
  \caption{Comparing UPV and $\text{UPV}_w$ in the scenario with 1\% outliers (1000 simulations).}
  \label{fig:upv1}
\end{figure}

\begin{figure}[h]
  \centering
  \includegraphics[width=.7\linewidth]{images/upv_w_0.05.png}
  \caption{Comparing UPV and $\text{UPV}_w$ in the scenario with 5\% outliers (1000 simulations).}
  \label{fig:upv5}
\end{figure}

\section{Presence of outliers in the initial design}\label{app:b}

In this section, we investigate the impact of removing the assumption that the initial design is free from outliers on the sampling strategies. Despite the small size of the initial design when $p=20$, we observed several notable behaviors. One of the most noticeable differences is that the learning curves start with higher errors, as there are outliers forcibly included in the data. However, over time, the learning curves of the robust strategies are able to converge to satisfactory predictive performance as they can minimize the impact of these observations on the model training. In contrast, the OLS-based bounded CDO performs significantly worse in this scenario. This is because estimating the cutoff value $\Gamma_2$ using a contaminated set does not provide adequate protection against the inclusion of outliers in the design.

\begin{figure}[H]
  \centering
  \includegraphics[width=.7\linewidth]{images/0.00275_dirty.png}
  \caption{Comparing query strategies with 0.275\% outliers (1000 simulations). Plots (b) and (d) offer a closer view on the two best strategies from plots (a) and (c), respectively, with shaded regions indicating the standard deviation across the simulations.}
  \label{fig:0275dirty}
\end{figure}

\begin{figure}[H]
  \centering
  \includegraphics[width=.7\linewidth]{images/0.01_dirty.png}
  \caption{Comparing query strategies with 1\% outliers (1000 simulations): results from 1000 simulations. Plots (b) and (d) offer a closer view on the two best strategies from plots (a) and (c), respectively, with shaded regions indicating the standard deviation across the simulations.}
  \label{fig:001dirty}
\end{figure}

\begin{figure}[H]
  \centering
  \includegraphics[width=.7\linewidth]{images/0.05_dirty.png}
  \caption{Comparing query strategies with 5\% outliers (1000 simulations): results from 1000 simulations. Plots (b) and (d) offer a closer view on the two best strategies from plots (a) and (c), respectively, with shaded regions indicating the standard deviation across the simulations.}
  \label{fig:005dirty}
\end{figure}
